# Supplementary material for: A Survey on ML4VIS: Applying Machine Learning Advances to Data Visualization
Source: arXiv:2012.00467 source file (2021-12-23)
Supplement: Supplementary file 1 [file supp_crop.pdf]

| ID | paper name                  | venue    | year | field | VIS CODE                   |                            |                                  | ML CODE         |                                  |                             |                            |               |  |
|----|-----------------------------|----------|------|-------|----------------------------|----------------------------|----------------------------------|-----------------|----------------------------------|-----------------------------|----------------------------|---------------|--|
|    |                             |          |      |       | vis-driven data processing | communicate / present data | VIS perception / imitate insight | VIS interaction | dimension reduction / clustering | classification / generative | semi-supervised regression | reinforcement |  |
| 1  | Behavior-Driven Visualizat  | IUI      | 2009 | hci   |                            |                            |                                  |                 |                                  |                             |                            |               |  |
| 2  | Revision: Automated class   | UIST     | 2011 | hci   |                            |                            |                                  |                 |                                  |                             |                            |               |  |
| 3  | VizDeck: self-organizing d  | SIGMOD   | 2012 | dm    |                            |                            |                                  |                 |                                  |                             |                            |               |  |
| 4  | User-Adaptive Information   | IUI      | 2013 | hci   |                            |                            |                                  |                 |                                  |                             |                            |               |  |
| 5  | Prediction of Users' Learni | IUI      | 2014 | hci   |                            |                            |                                  |                 |                                  |                             |                            |               |  |
| 6  | Towards facilitating user s | IUI      | 2014 | hci   |                            |                            |                                  |                 |                                  |                             |                            |               |  |
| 7  | Finding waldo: Learning at  | TVCG     | 2014 | vis   |                            |                            |                                  |                 |                                  |                             |                            |               |  |
| 8  | Data-driven evaluation of \ | CGF      | 2015 | vis   |                            |                            |                                  |                 |                                  |                             |                            |               |  |
| 9  | FigureSeer: Parsing Resul   | ECCV     | 2016 | ml    |                            |                            |                                  |                 |                                  |                             |                            |               |  |
| 10 | A Diagram Is Worth A Doz    | ECCV     | 2016 | ml    |                            |                            |                                  |                 |                                  |                             |                            |               |  |
| 11 | Automatic Summary Gene      | aaai     | 2016 | ml    |                            |                            |                                  |                 |                                  |                             |                            |               |  |
| 12 | Towards Visualization Rec   | SIGMOD   | 2016 | dm    |                            |                            |                                  |                 |                                  |                             |                            |               |  |
| 13 | SepMe: 2002 New Visual §    | PVis     | 2016 | vis   |                            |                            |                                  |                 |                                  |                             |                            |               |  |
| 14 | VizRec: Recommending p      | TiiS     | 2016 | hci   |                            |                            |                                  |                 |                                  |                             |                            |               |  |
| 15 | A machine learning approæ   | aaai     | 2017 | ml    |                            |                            |                                  |                 |                                  |                             |                            |               |  |
| 16 | See Without Looking: Joint  | IJCAI    | 2017 | ml    |                            |                            |                                  |                 |                                  |                             |                            |               |  |
| 17 | Foresight: Recommending     | VLDB     | 2017 | dm    |                            |                            |                                  |                 |                                  |                             |                            |               |  |
| 18 | Extracting and Retargeting  | IEEE VIS | 2017 | vis   |                            |                            |                                  |                 |                                  |                             |                            |               |  |
| 19 | What Would a Graph Look     | IEEE VIS | 2017 | vis   |                            |                            |                                  |                 |                                  |                             |                            |               |  |
| 20 | Graph Layouts by t-SNE      | EuroVis  | 2017 | vis   |                            |                            |                                  |                 |                                  |                             |                            |               |  |
| 21 | Reverse-Engineering Visu    | EuroVis  | 2017 | vis   |                            |                            |                                  |                 |                                  |                             |                            |               |  |
| 22 | Learning Visual Importanc   | UIST     | 2017 | hci   |                            |                            |                                  |                 |                                  |                             |                            |               |  |
| 23 | Understanding Infographic   | arxiv    | 2017 | other |                            |                            |                                  |                 |                                  |                             |                            |               |  |
| 24 | ChartSense: Interactive D   | CHI      | 2017 | hci   |                            |                            |                                  |                 |                                  |                             |                            |               |  |
| 25 | DVQA: Understanding Dat     | CVPR     | 2018 | ml    |                            |                            |                                  |                 |                                  |                             |                            |               |  |
| 26 | Dynamic Graph Generatio     | CVPR     | 2018 | ml    |                            |                            |                                  |                 |                                  |                             |                            |               |  |
| 27 | JUMP: A Joint Predictor fo  | IJCAI    | 2018 | ml    |                            |                            |                                  |                 |                                  |                             |                            |               |  |
| 28 | FIGUREQA: AN ANNOTA         | ICLR     | 2018 | ml    |                            |                            |                                  |                 |                                  |                             |                            |               |  |
| 29 | Next-Step Suggestions for   | KDD      | 2018 | dm    |                            |                            |                                  |                 |                                  |                             |                            |               |  |
| 30 | DeepEye: Towards Autom      | ICDE     | 2018 | dm    |                            |                            |                                  |                 |                                  |                             |                            |               |  |
| 31 | ShapeSearch: Flexible Pat   | VLDB     | 2018 | dm    |                            |                            |                                  |                 |                                  |                             |                            |               |  |
| 32 | DeepEye: Creating Good I    | SIGMOD   | 2018 | dm    |                            |                            |                                  |                 |                                  |                             |                            |               |  |
| 33 | An Analysis of Automated    | IEEE VIS | 2018 | vis   |                            |                            |                                  |                 |                                  |                             |                            |               |  |
| 34 | Formalizing Visualization   | IEEE VIS | 2018 | vis   |                            |                            |                                  |                 |                                  |                             |                            |               |  |
| 35 | A Generative Model for Vo   | IEEE VIS | 2018 | vis   |                            |                            |                                  |                 |                                  |                             |                            |               |  |
| 36 | A Perception-Driven Apprc   | IEEE VIS | 2018 | vis   |                            |                            |                                  |                 |                                  |                             |                            |               |  |
| 37 | Evaluating 'Graphical Perc  | IEEE VIS | 2018 | vis   |                            |                            |                                  |                 |                                  |                             |                            |               |  |
| 38 | Fast and accurate CNN-b     | EuroVis  | 2018 | vis   |                            |                            |                                  |                 |                                  |                             |                            |               |  |
| 39 | Interactive Visual Explorat | EuroVis  | 2018 | vis   |                            |                            |                                  |                 |                                  |                             |                            |               |  |
| 40 | Beagle: Automated Extrac    | CHI      | 2018 | hci   |                            |                            |                                  |                 |                                  |                             |                            |               |  |
| 41 | Predicting Human Perform    | CHI      | 2018 | hci   |                            |                            |                                  |                 |                                  |                             |                            |               |  |
| 42 | Data Interpretation and Re  | arxiv    | 2018 | other |                            |                            |                                  |                 |                                  |                             |                            |               |  |
| 43 | Data2Vis: Automatic Gene    | CGA      | 2018 | vis   |                            |                            |                                  |                 |                                  |                             |                            |               |  |
| 44 | Synthetically Trained Icon  | arxiv    | 2018 | other |                            |                            |                                  |                 |                                  |                             |                            |               |  |

|    |                             |          |      |       |                                 |
|----|-----------------------------|----------|------|-------|---------------------------------|
| 45 | Evaluating the Readability  | CGA      | 2018 | vis   |                                 |
| 46 | FlowSense: A Natural Lan    | IEEE VIS | 2019 | vis   |                                 |
| 47 | InSituNet: Deep Image Syri  | IEEE VIS | 2019 | vis   |                                 |
| 48 | LassoNet: Deep Lasso-SeI    | IEEE VIS | 2019 | vis   |                                 |
| 49 | TSR-TVD: Temporal Supe      | IEEE VIS | 2019 | vis   |                                 |
| 50 | GenerativeMap: Visualizat   | IEEE VIS | 2019 | vis   |                                 |
| 51 | A Deep Generative Model     | IEEE VIS | 2019 | vis   |                                 |
| 52 | DeepDrawing: A Deep Lea     | IEEE VIS | 2019 | vis   |                                 |
| 53 | FlowNet: A Deep Learning    | IEEE VIS | 2019 | vis   |                                 |
| 54 | A Markov Model of Users'    | IEEE VIS | 2019 | vis   |                                 |
| 55 | An Incremental Dimension    | IEEE VIS | 2019 | vis   |                                 |
| 56 | Visualization Assessment:   | IEEE VIS | 2019 | vis   |                                 |
| 57 | A Deep Learning Approach    | IEEE VIS | 2019 | vis   |                                 |
| 58 | Disentangled Representat    | IEEE VIS | 2019 | vis   |                                 |
| 59 | ScatterNet: A Deep Subjec   | IEEE VIS | 2019 | vis   |                                 |
| 60 | DataShot: Automatic Gene    | IEEE VIS | 2019 | vis   |                                 |
| 61 | Text-to-Viz: Automatic Ge   | IEEE VIS | 2019 | vis   |                                 |
| 62 | Towards Automated Infog     | IEEE VIS | 2019 | vis   |                                 |
| 63 | DeepOrganNet: On-the-FI     | IEEE VIS | 2019 | vis   |                                 |
| 64 | Color Crafting: Automating  | IEEE VIS | 2019 | vis   |                                 |
| 65 | A Natural-language-based    | IEEE VIS | 2019 | vis   |                                 |
| 66 | On KDE-based brushing ir    | EuroVis  | 2019 | vis   |                                 |
| 67 | Follow The Clicks: Learnin  | EuroVis  | 2019 | vis   |                                 |
| 68 | ClustMe: A Visual Quality I | EuroVis  | 2019 | vis   |                                 |
| 69 | Online Learning of Visualiz | EuroVis  | 2019 | vis   |                                 |
| 70 | DNN-VolVis: Interactive V   | PVis     | 2019 | vis   |                                 |
| 71 | Answering Questions abou    | arxiv    | 2019 | other |                                 |
| 72 | Interactive Cleaning for Pr | ICDE     | 2020 | dm    |                                 |
| 73 | ICONATE: Automatic Corr     | CHI      | 2020 | hci   |                                 |
|    |                             |          |      |       | 4 13 4 6 27 19 3 6 13 36 14 0 1 |
